# Supplementary material for: Support-based lower bounds for the positive semidefinite rank of a nonnegative matrix
Source: arXiv:1203.3961 source file (2013-11-15)
Supplement: Supplementary file 1 [file appendix.tex]

% support-lbs/appendix.tex

\appendix
\section{Linear extensions of the cut polytope dominating the clique inequalities}\label{apx:linear-cut-clique}

Here we prove Remark~\ref{rem:linear-cut-clique}.  Let $P_0$ denote the cut polytope of a complete graph on~$n$ vertices, and let~$P_1^c$ as defined on
page~\pageref{page:def-clique-relax}.

We quickly repeat some definitions from graph theory.  Let~$G$ be a bipartite graph with vertex set $X\amalg Y$ (here, and in what follows, $\amalg$ stands for the
disjoint union of two not necessarily disjoint sets).  A \textit{biclique} in~$G$ is a complete bipartite graph with vertex set $U\amalg V$, for sets $U\subseteq X$,
$V\subseteq Y$, which is a subgraph of~$G$.  We say that biclique~$B$ \textit{covers} an edge $(u,v)\in E(G)$, if $(u,v)\in E(B)$.  The \textit{biclique covering
  number} is the minimum number of bicliques in~$G$ required to cover all edges of~$G$.

As mentioned in the introduction, the biclique covering number is just the Boolean rank of the Boolean $X\times Y$-matrix~$M$ with $M(x,y) = 1$ if and only if
$(x,y) \in E(G)$.  It is a lower bound to the nonnegative rank of any matrix~$S$ with $\supp S = M$.

% \newcommand{\powN}{2^{[N]}}%
% Denoting the power set of the set $\{1,\dots,N\}$ by $\powN$, let $H$ denote the bipartite graph with vertex set $\powN\amalg\powN$, and $(x,y) \in E(H)$ if and
% only if $x\cap y = \emptyset$.  Let~$\bar H$ denote the bipartite graph on the same vertex set and with $(x,y) \in E(\bar H)$ if and only if $\abs{x\cap y} = 1$
% (so $E(\bar H) \cap E(H) = \emptyset$).  A biclique is called \textit{$\bar H$-feasible,} if it contains no edge of~$\bar H$.  (It may, however, contain edges
% which are neither in $H$ nor in~$\bar H$, i.e., it might not a biclique in~$H$.)
To lower bound the biclique covering number, we will use a lower bound on the communication complexity of the {\em unique disjointness} problem.  For strings $x,y$
of length $N$, the unique disjointness function evaluates to $1$ if $x \cap y = \emptyset$ and evaluates to $0$ if $|x \cap y|=1$.  Otherwise, it is undefined.
The specific result we will need is an exponential lower bound on the number of bicliques to cover the ones of unique disjointness, provided that no biclique
covers a zero of the function.  This lower bound follows simply from the key lemma of Razborov~\cite{Razborov92} used to prove an $\Omega(n)$ lower bound on the
randomized communication complexity of disjointness, and is explicitly stated in~\cite{deWolf03}.  For a textbook treatment, see
Lemma~4.49 in Kushilevitz \& Nisan~\cite{KushilevitzNisan97}.

\newcommand{\bse}{\binom{[N]}{\ell}}%
We now more precisely state the exact result we need.  Let~$N=4\ell+1$ be an odd integer.  Denoting the set of all $\ell$-element subsets of $\{1,\dots,N\}$ by
$\bse$, let $H_N$ denote the bipartite graph with vertex set $\bse\amalg\bse$, and $(x,y) \in E(H_N)$ if and only if $x\cap y = \emptyset$.  Let~$\bar H_N$ denote
the bipartite graph on the same vertex set and with $(x,y) \in E(\bar H_N)$ if and only if $\abs{x\cap y} = 1$ (so $E(\bar H_N) \cap E(H_N) = \emptyset$).  A
biclique is called \textit{$\bar H_N$-feasible,} if it contains no edge of~$\bar H_N$.  (It may, however, contain edges which are neither in $H_N$ nor in~$\bar
H_N$, i.e., it might not be a biclique in~$H_N$.)

%In communication complexity, the question how many $\bar H_N$-feasible bicliques are needed to cover all edges of~$H_N$ is related to the randomized communication
%complexity of the so-called 1-disjointness function, which was first computed by~\cite{KalyanasundaramSchnitger92}.  The following result is an easy corollary of
%this result in the version of Lemma~4.49 in the book by Kushilevitz \& Nisan~\cite{KushilevitzNisan97}.

\begin{theorem}[\cite{Razborov92, deWolf03}]\label{thm:1dj}
  The number of $\bar H_N$-feasible bicliques needed to cover all edges in~$H_N$ is $\displaystyle 2^{\Omega(N)}$.
\end{theorem}

This theorem was used in~\cite{FioriniMassarPokuttaTiwaryDewolf2012} to prove their main result.  Our usage is different, though.

\begin{proof}[Proof of Remark~\ref{rem:linear-cut-clique}]
  By Theorem~\ref{thm:nnegrk-lext}, we have to prove that the slack matrix for the relaxation $P_0 \subset P_1^c$ has nonnegative rank $2^{\Omega(n)}$.  The
  approach is to bound the Boolean rank.  For this, we will give a lower bound to the biclique covering number of the following bipartite graph~$G$.  The vertices
  of~$G$ are, on the one hand, the cliques~$U$, $U\subset V_n$, and on the other hand the cuts $\delta(W)$, $W\subset V_n$.  We have $(U,\delta(W)) \in E(G)$ if and
  only if $\abs{U\cap \delta(W)} < \nfrac{\abs{U}^2}{4}$.  In other words, there is \textsl{no} edge between $U$ and $\delta(W)$, if and only if $\abs{ U\cap W } =
  \abs{U}/2$.

  We make no attempt to optimize the constant in the exponent.

  Assuming that $n=2 \bmod 8$, let $N := n/2$, $\ell := \lfloor N/4 \rfloor$.  Given a list of~$r$ bicliques in~$G$ which cover every edge of~$G$, we construct a
  covering of the edges of~$H_N$ by (at most) $r$ bicliques which are $\bar H_N$-feasible.  Consider the sets $U$ with cardinality $2\ell-2$ which have $U\cap
  \{N+1,\dots,n\} = \{N+1,\dots,N+\ell-2\}$, and the sets~$W$ of cardinality $u$ which satisfy $U\cap \{N+1,\dots,n\} = \{N+1,\dots,N+\ell-2\}$, too.  Then
  $\abs{U\cap W} = \nfrac{\abs{U}}{2} = \ell-1$ if and only if the two $\ell$-element sets $x := U\cap \{1,\dots,N\}$ and $y := W\cap \{1,\dots,N\}$ satisfy
  $\abs{x\cap y} = 1$.  Thus, a covering of the the edges of the subgraph of~$G$ spanned by this type of vertices $U$ and~$\delta(W)$ of~$G$ by bicliques in~$G$
  gives a covering of the edges of~$H_N$ by $\bar H_N$-feasible bicliques.  By Theorem~\ref{thm:1dj}, such a covering must have $2^{\Omega(n)}$ bicliques.
\end{proof}

%%% Local Variables: 
%%% mode: latex
%%% TeX-master: "support-lbs.tex"
%%% fill-column: 164
%%% End: 
